# Supplementary material for: Robust Semi-supervised Learning by Wisely Leveraging Open-set Data
Source: arXiv:2405.06979 source file (2024-05-20)
Supplement: Supplementary file 1 [file Appendix.tex]

\appendices
\section{Proof of the Theorem 1}

\begin{proof}
(a) Following the standard analysis, we have the following inequality in expectation
\begin{align}\label{thm:1:eq:1}
\nonumber&\E[\Lmath(\theta_{t+1}) - \Lmath(\theta_t)] \\
\nonumber\overset{(\text{i})}{\le} &\E[ \langle \theta_{t+1} - \theta_t, \nabla \Lmath(\theta_t)\rangle] + \frac{L}{2}\E[\|\theta_{t+1} - \theta_t\|^2]\\
\nonumber\overset{(\text{ii})}{=}& -\eta\E[\langle \gt(\theta_t), \nabla \Lmath(\theta_t)\rangle] + \frac{\eta^2 L}{2}\E[\|\gt(\theta_t)\|^2] \\
%=& \frac{\eta}{2}\E[\|\nabla \Lmath(\theta_t) - \gt(\theta_t)\|^2]- \frac{\eta}{2}\left(\|\nabla \Lmath(\theta_t)\|^2 + \left(1 - \eta L\right)\E[\|\gt(\theta_t)\|^2] \right), 
\nonumber\overset{(\text{iii})}{=}&-\eta(1- \frac{\eta L}{2})\|\nabla \Lmath(\theta_t)\|^2 + \frac{\eta^2L}{2}\E[\|\nabla \Lmath(\theta_t) - \gt(\theta_t)\|^2]\\
\overset{(\text{iv})}{\le}&- \frac{\eta}{2}\|\nabla \Lmath(\theta_t)\|^2 + \frac{\eta^2L}{2}\E[\|\nabla \Lmath(\theta_t) - \gt(\theta_t)\|^2],
\end{align}
where (i) is due to the smoothness of loss function $\Lmath$ in Assumption~\ref{ass:smooth}; (ii) is due to the update of SGD; (iii) is due to $\E[\gt(\theta)]=\nabla \Lmath(\theta)$; (iv) is due to $\eta \le 1/L$. By the definition of $\gt(\theta_t)$ and the convexity of norm $\|\cdot\|^2$, we know 
\begin{align}\label{thm:1:eq:2}
    \nonumber&\E[\|\nabla \Lmath(\theta_t) - \gt(\theta_t)\|^2] \\
    \nonumber\le &\lambda\E[\|\nabla \Lmath(\theta_t) - \gi(\theta_t)\|^2] \\
    \nonumber &+ (1-\lambda) (\tau \E[\|\nabla \Lmath(\theta_t) - \gn(\theta_t)\|^2 \\
    \nonumber &+ (1-\tau)\E[\|\nabla \Lmath(\theta_t) - \gf(\theta_t)\|^2])\\
    \nonumber\le & \lambda \sigma^2 + (1-\lambda) [\tau (\frac{\epsilon}{2}\|\nabla \Lmath(\theta_t)\|^2 +\sigma^2)\\
    \nonumber &+ (1-\tau)(\frac{\nu}{2}\|\nabla \Lmath(\theta_t) \|^2 + \sigma^2) ]\\
     = & \sigma^2 + (1-\lambda)\frac{\tau\epsilon + (1-\tau)\nu}{2}\|\nabla \Lmath(\theta_t)\|^2, 
\end{align}
where the second inequality is due to Assumptions~\ref{ass:grad} and \ref{ass:grad:Fb}. Therefore, by (\ref{thm:1:eq:1}) and (\ref{thm:1:eq:2}) we have
\begin{align}\label{thm:1:eq:3}
\nonumber&\E[\Lmath(\theta_{t+1}) - \Lmath(\theta_t)] \\
\nonumber\le& - \frac{\eta }{2}\left( 1 - \eta L(1-\lambda)\frac{\tau\epsilon + (1-\tau)\nu}{2} \right)\E[\|\nabla \Lmath(\theta_t)\|^2]+ \frac{\eta^2L\sigma^2}{2} \\
\le& - \frac{\mu \eta }{2}\E[\Lmath(\theta_t)-\Lmath(\theta_*)]+ \frac{\eta^2L\sigma^2}{2} ,
\end{align}
where the last inequality is due to  Assumption~\ref{ass:PL} and $\eta = \frac{1}{(1-\lambda)(\tau\epsilon + (1-\tau)\nu) L}$. Therefore, we have
\begin{align}\label{thm:1:eq:4}
\E[\Lmath(\theta_{t+1}) - \Lmath(\theta_*)] 
\le \left(1- \frac{\mu \eta }{2}\right)\E[\Lmath(\theta_t)-\Lmath(\theta_*)]+ \frac{\eta^2L\sigma^2}{2} ,
\end{align}
which implies 
\begin{align}\label{thm:1:eq:5}
\nonumber&\E[\Lmath(\theta_{n+m+m'+1}) - \Lmath(\theta_*)] \\
\le &\exp\left(-\mu \eta (n+m+m')/2 \right)(\Lmath(\theta_0)-\Lmath(\theta_*))+ \frac{\eta L\sigma^2}{\mu},
\end{align}
Since $\nu$ is large enough, then we know that $\eta' := \frac{1}{(1-\lambda)(\tau\epsilon + (1-\tau)\nu) L}$ is small enough such that $\exp\left(-\mu \eta' (n+m+m')/2 \right) \gg \frac{L\sigma^2}{(n+m+m')\mu^2 (\Lmath(\theta_0)-\Lmath(\theta_*))}$. 
Thus, we have
\begin{align}\label{thm:1:eq:6}
\nonumber &\E[\Lmath(\theta_{n+m+m'+1}) - \Lmath(\theta_*)] \\
\le & \exp\left(-\mu \eta' (n+m+m')/2 \right)(\Lmath(\theta_0)-\Lmath(\theta_*))+ \frac{\eta' L\sigma^2}{\mu}
\end{align}
Let's consider a special case of $ n+m+m' = \frac{2(1-\lambda)(\tau\epsilon + (1-\tau)\nu) L}{\mu}$, then $\eta' = \frac{2}{(n+m+m')\mu}$, implying
\begin{align}\label{thm:1:eq:6:2}
\E[\Lmath(\theta_{n+m+m'+1}) - \Lmath(\theta_*)] \le  O\left(\Lmath(\theta_0)-\Lmath(\theta_*)\right)
\end{align}

(b) Next, let's consider the case without either far OOD data or near OOD data, i.e., $\lambda= 1$. Then, following the similar analysis in (a), we have
\begin{align}\label{thm:1:eq:11}
\nonumber&\E[\Lmath(\theta_{t+1}) - \Lmath(\theta_t)] \\
\nonumber\le& - \frac{\eta }{2}\E[\|\nabla \Lmath(\theta_t)\|^2]+ \frac{\eta^2L\sigma^2}{2} \\
\le& - \frac{\mu \eta }{2}\E[\Lmath(\theta_t)-\Lmath(\theta_*)]+ \frac{\eta^2L\sigma^2}{2} ,
\end{align}
where the last inequality is due to  Assumption~\ref{ass:PL}. Therefore, we have
\begin{align}\label{thm:1:eq:8}
\E[\Lmath(\theta_{t+1}) - \Lmath(\theta_*)] 
\le \left(1- \frac{\mu \eta }{2}\right)\E[\Lmath(\theta_t)-\Lmath(\theta_*)]+ \frac{\eta^2L\sigma^2}{2} ,
\end{align}
which implies 
\begin{align}\label{thm:1:eq:9}
\E[\Lmath(\theta_{n+1}) - \Lmath(\theta_*)] 
\le \exp\left(-\mu \eta n/2 \right)(\Lmath(\theta_0)-\Lmath(\theta_*))+ \frac{\eta L\sigma^2}{\mu},
\end{align}
By setting $\eta = \frac{2}{n\mu} \log\left( \frac{n\mu^2(\Lmath(\theta_0)-\Lmath(\theta_*))}{\sigma^2L}\right)$,
\begin{align}\label{thm:1:eq:10}
\nonumber&\E[\Lmath(\theta_{n+1}) - \Lmath(\theta_*)]  \\
\nonumber\le &\frac{L\sigma^2}{n\mu^2}+ \frac{2L\sigma^2}{n\mu^2} \log\left( \frac{n\mu^2(\Lmath(\theta_0)-\Lmath(\theta_*))}{\sigma^2L}\right)\\
\le & O\left( \frac{\log\left( n \right)}{n}  \right)
\end{align}

(c) Finally, let's consider the case without far OOD data (but with near OOD data), i.e., $\tau= 1$. Then, following the similar analysis in (a), we have
\begin{align}\label{thm:1:eq:7}
\nonumber&\E[\Lmath(\theta_{t+1}) - \Lmath(\theta_t)] \\
\nonumber\le& - \frac{\eta }{2}\left( 1 - \frac{(1-\lambda)\epsilon \eta L }{2} \right)\E[\|\nabla \Lmath(\theta_t)\|^2]+ \frac{\eta^2L\sigma^2}{2} \\
\le& - \frac{\mu \eta }{2}\E[\Lmath(\theta_t)-\Lmath(\theta_*)]+ \frac{\eta^2L\sigma^2}{2},
\end{align}
where the last inequality is due to  Assumption~\ref{ass:PL} and $\eta \le \frac{1}{(1-\lambda)\epsilon \nu L}$. Therefore, we have
\begin{align}\label{thm:1:eq:8}
\E[\Lmath(\theta_{t+1}) - \Lmath(\theta_*)] 
\le \left(1- \frac{\mu \eta }{2}\right)\E[\Lmath(\theta_t)-\Lmath(\theta_*)]+ \frac{\eta^2L\sigma^2}{2} ,
\end{align}
which implies 
\begin{align}\label{thm:1:eq:9}
\small
\nonumber& \E[\Lmath(\theta_{n+m+1}) - \Lmath(\theta_*)] \\
\le & \exp\left(-\mu \eta (n+m)/2 \right)(\Lmath(\theta_0)-\Lmath(\theta_*))+ \frac{\eta L\sigma^2}{\mu},
\end{align}
By setting $\eta = \frac{2}{(n+m)\mu} \log\left( \frac{(n+m)\mu^2(\Lmath(\theta_0)-\Lmath(\theta_*))}{\sigma^2L}\right)$,
\begin{align}\label{thm:1:eq:10}
\nonumber&\E[\Lmath(\theta_{n+m+1}) - \Lmath(\theta_*)]  \\
\nonumber\le &\frac{L\sigma^2}{(n+m)\mu^2}+ \frac{2L\sigma^2}{(n+m)\mu^2} \log\left( \frac{(n+m)\mu^2(\Lmath(\theta_0)-\Lmath(\theta_*))}{\sigma^2L}\right)\\
\le & O\left( \frac{\log\left( n+m \right)}{(n+m)}  \right)
\end{align}

\end{proof}
